# Supplementary material for: Dissecting Service Mesh Overheads
Source: arXiv:2207.00592 source file (2022-07-02)

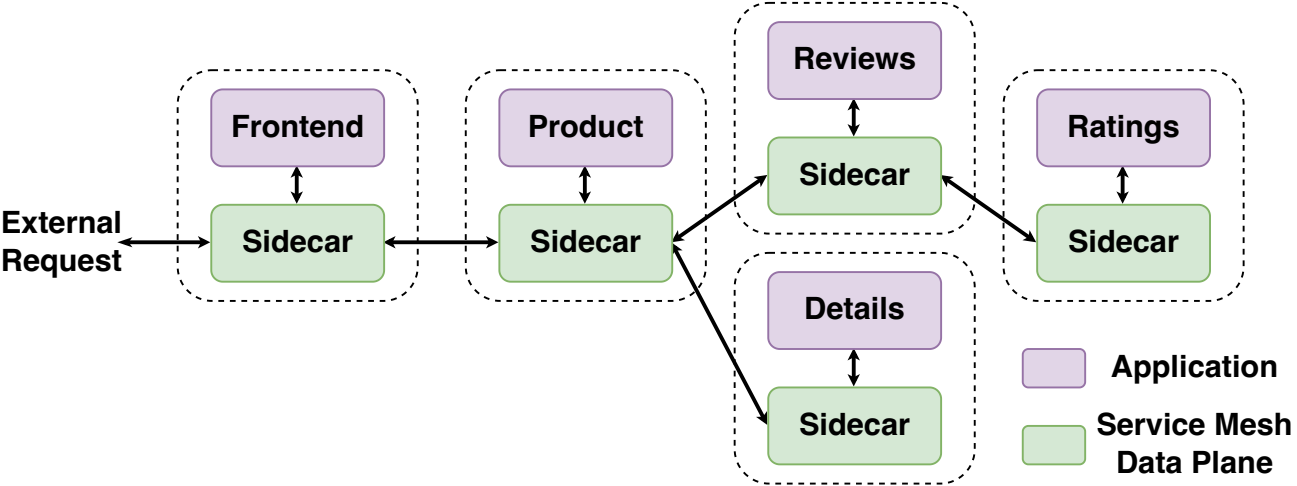

Supplement: Supplementary file 1 [file sm-arch.pdf]
